# Supplementary material for: Reversible Decoupling Network for Single Image Reflection Removal
Source: arXiv:2410.08063 source file (2025-03-31)
Supplement: Supplementary file 1 [file X_suppl.tex]

\clearpage
\setcounter{page}{1}
\maketitlesupplementary

\section{Further discussion about the TAPG}
\label{sec:rationale}
\label{sec:tapg}
\begin{figure}[h]
    \centering
\includegraphics[width=0.4\textwidth]{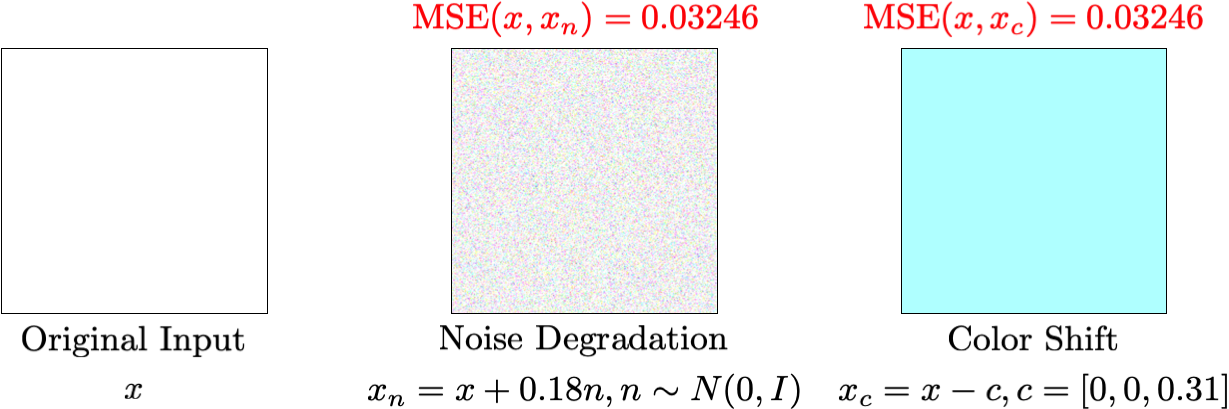}
    \caption{Visualization of the drawback of Mean Squared Error (MSE). Both color shifts and noise degradation exhibit the same MSE  relative to the ground truth. }
    \label{fig:mse}
    %\vspace{-30pt}
\end{figure}
As illustrated in Fig.~\ref{fig:mse} with a toy visualization of a pure white image which we mentioned in Sec.~\ref{sec:mse}, even though the color bias and noise exhibit the same Mean Squared Error (MSE) relative to the ground truth,  a linear estimation can instantly correct the image's color shift, whereas noise requires more complex operations to address. Metrics like MSE and Mean Absolute Error (MAE) struggle to compel the network to effectively recognize and rectify the linear degradation in the physical formulations. 
In this context, by pre-calibrating the features with a transmission-rate-aware prompt, we can significantly mitigate the effects of linear degradation, such as color and intensity inconsistencies.

\section{Qualitative Comparisons}
  \textbf{More visual cases.} We exhibit a total of nine additional cases: two cases from the Real20 dataset in Fig.~\ref{fig:real_appen}, two cases from the Objects dataset in Fig.~\ref{fig:Solid_appen}, three cases from the Postcard dataset in Fig.~\ref{fig:Post_appen} and two real-world cases captured by us in Fig.~\ref{fig:our_appen}. As illustrated, our method excels at revealing the information obscured by reflections and is highly effective in removing the majority of the reflections.

\section{Additional Experiments}

\textbf{Quantitative result of nature dataset.} Quantitative results of various methods on nature dataset is presented in Tab. \ref{tab:nature}. Nature dataset consists of 20 real-world samples. Our method achieved the best PSNR and the second-best SSIM, with a marginal decrease of only 0.004 in SSIM. These results further underscore the superiority of our approach in real-world scenarios.

\begin{figure*}[t]
    \centering
    \includegraphics[width=\linewidth,height=3.5cm]{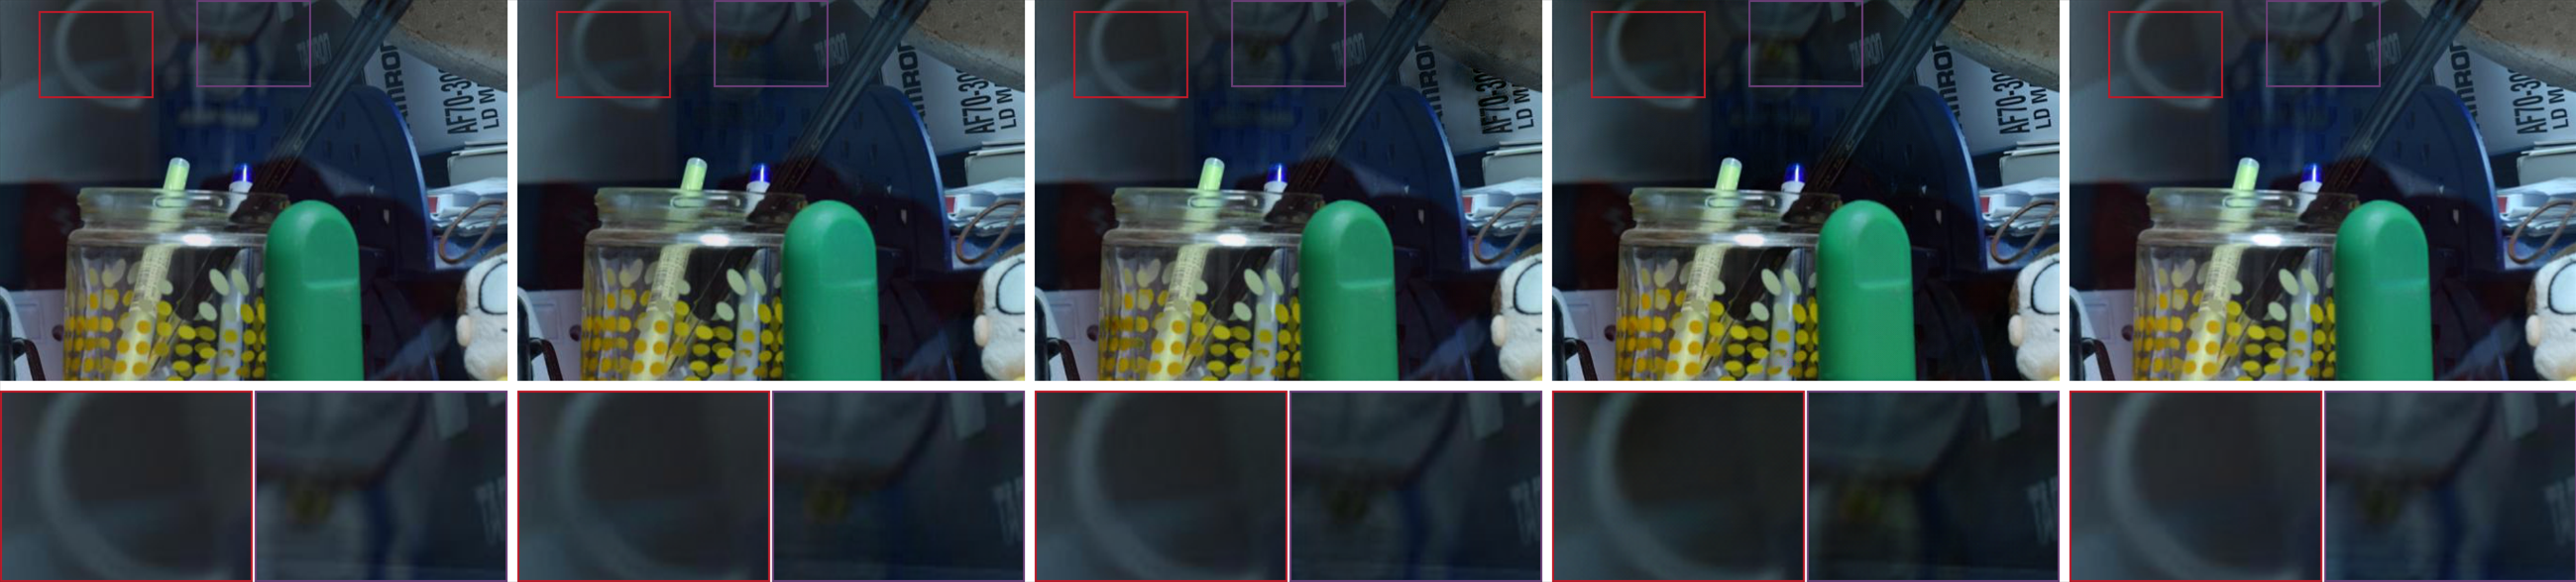} 
    \includegraphics[width=\linewidth,height=3.5cm]{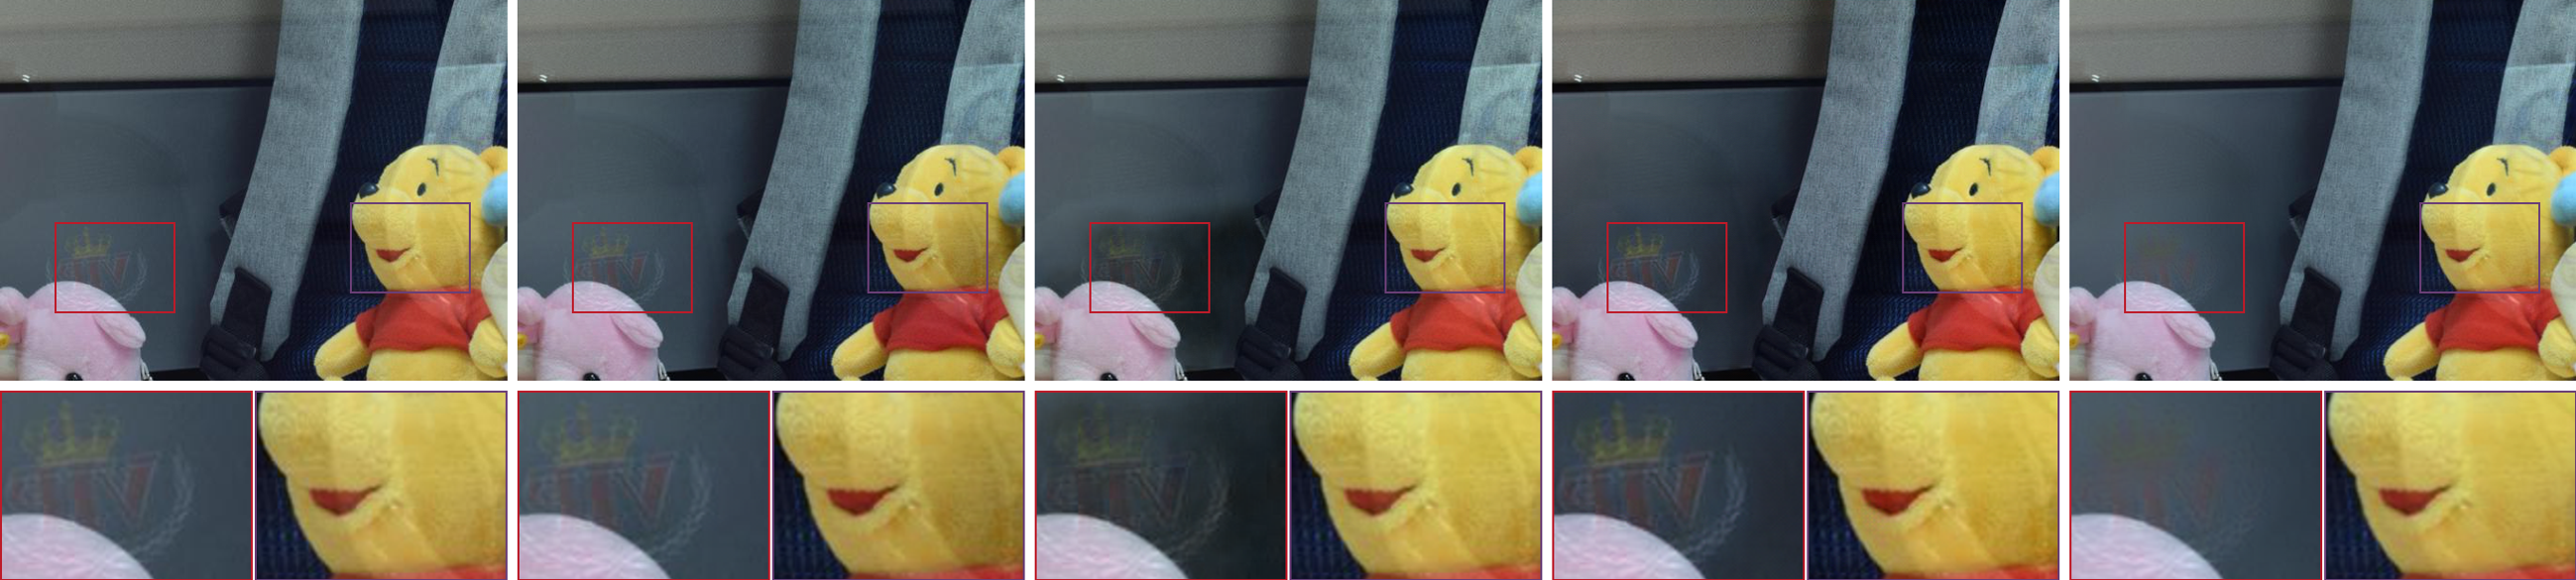}
    \includegraphics[width=\linewidth,height=3.5cm]{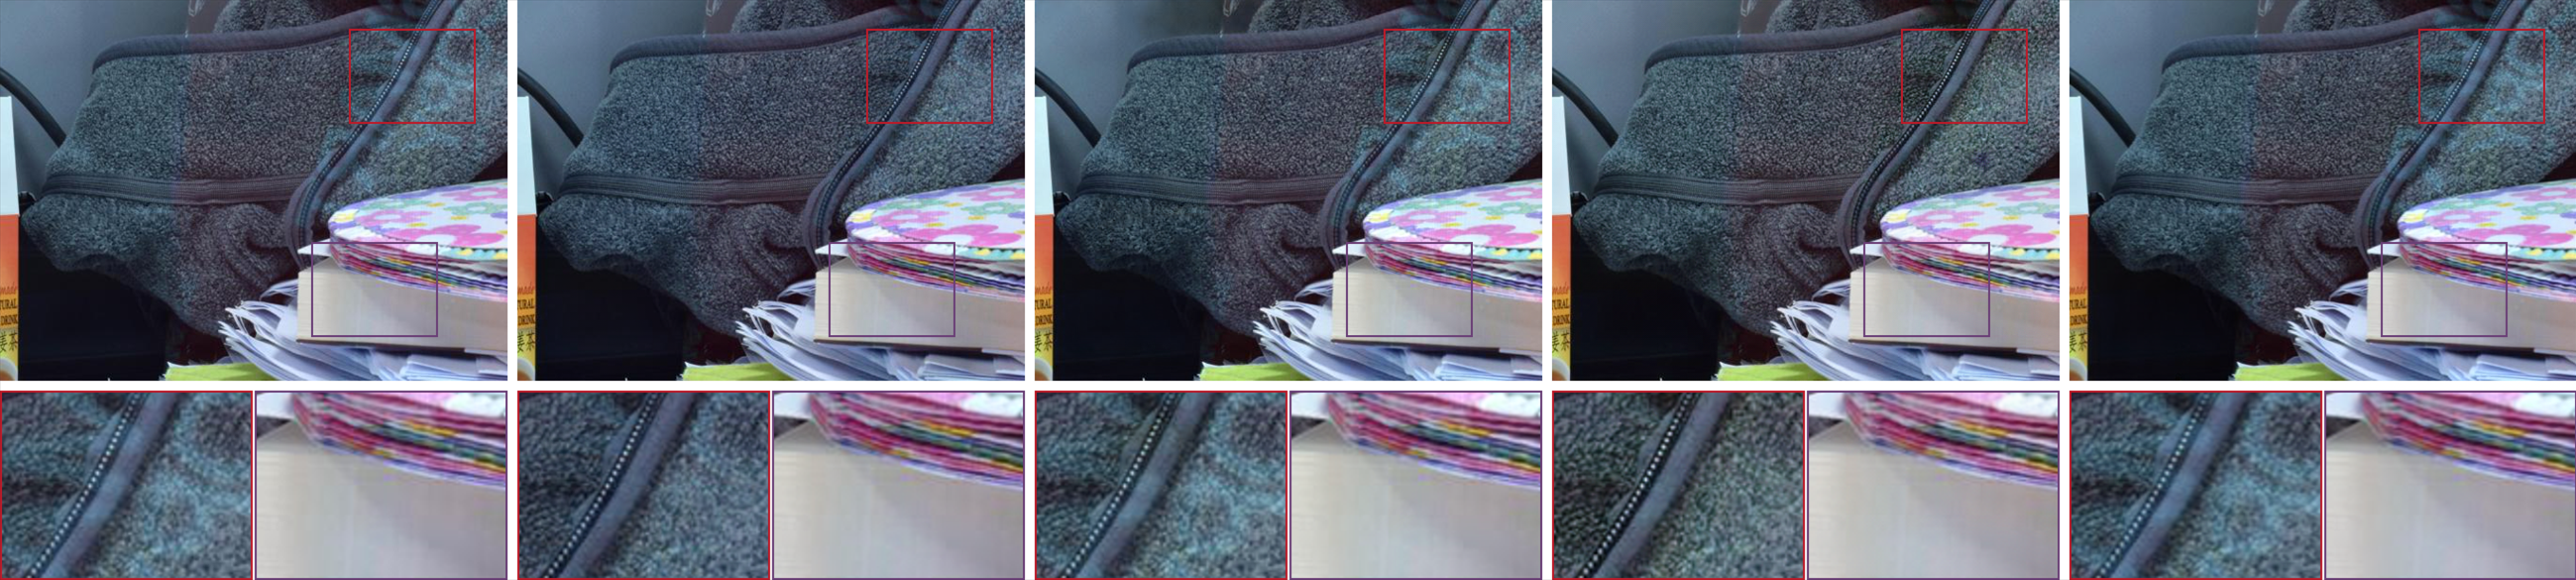}
    \begin{subfigure}{0.19\linewidth}
        \centering
        \subcaption{Input}
        \label{subfig:input}
    \end{subfigure}
    \begin{subfigure}{0.19\linewidth}
        \centering
        \subcaption{ERRNet}
        \label{subfig:ERRNet}
    \end{subfigure}
    \begin{subfigure}{0.19\linewidth}
        \centering
        \subcaption{IBCLN}
        \label{subfig:IBCLN}
    \end{subfigure}
    \begin{subfigure}{0.19\linewidth}
        \centering
        \subcaption{RAGNet}
        \label{subfig:RAGNet}
    \end{subfigure}
    \begin{subfigure}{0.19\linewidth}
        \centering
        \subcaption{Dong \textit{et al.}}
        \label{subfig:Dong}
    \end{subfigure}
    
    \includegraphics[width=\linewidth,height=3.5cm]{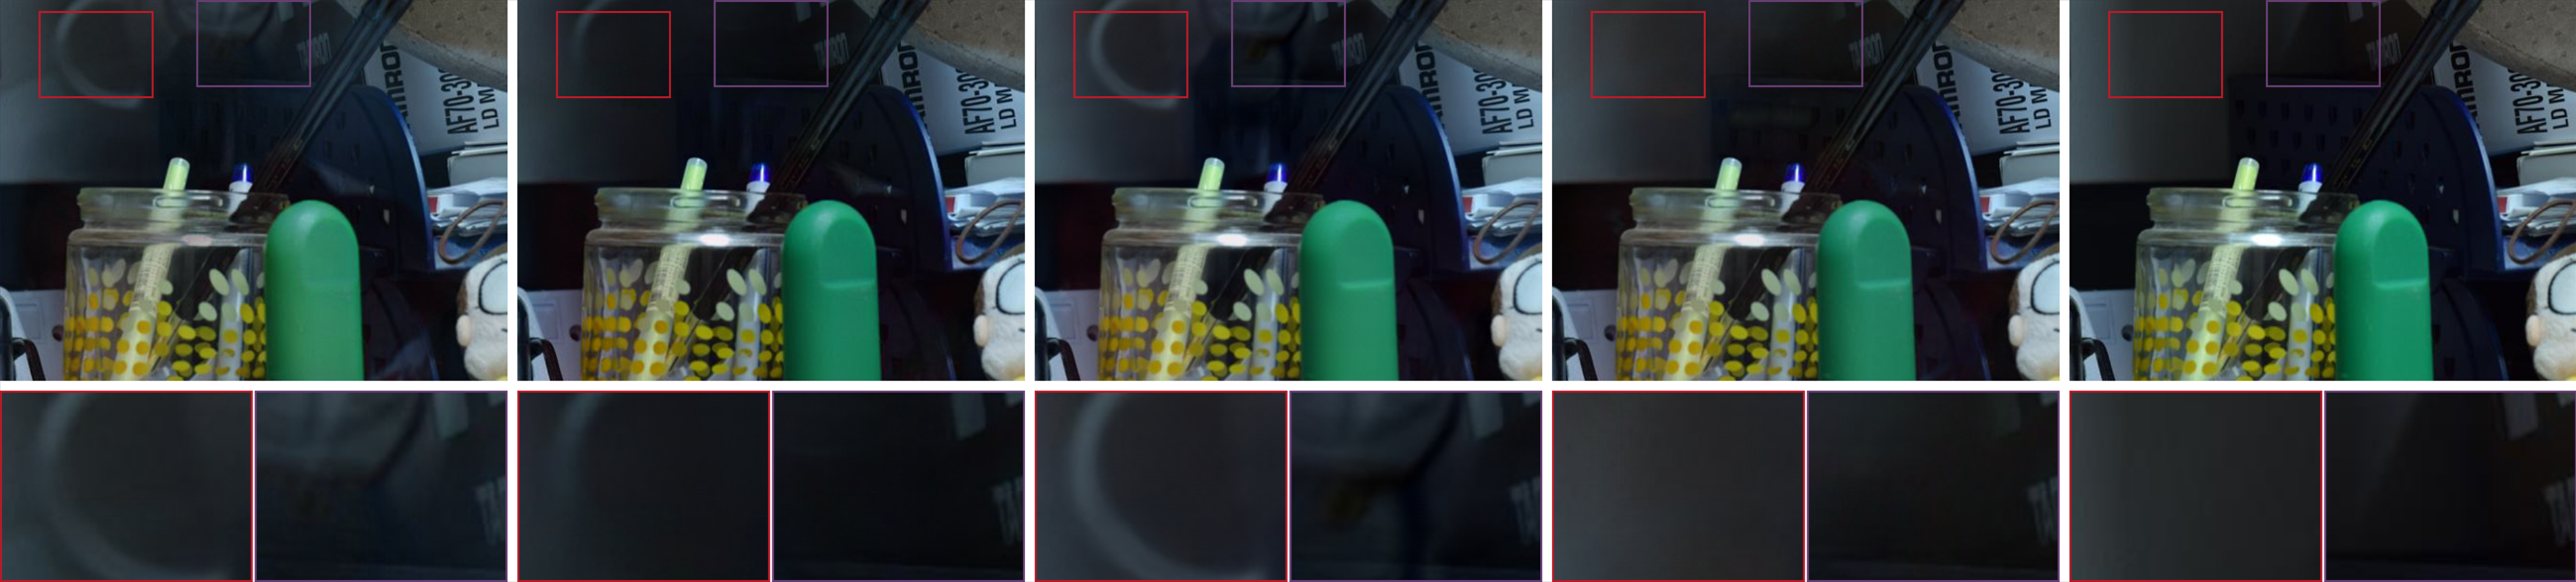}
    \includegraphics[width=\linewidth,height=3.5cm]{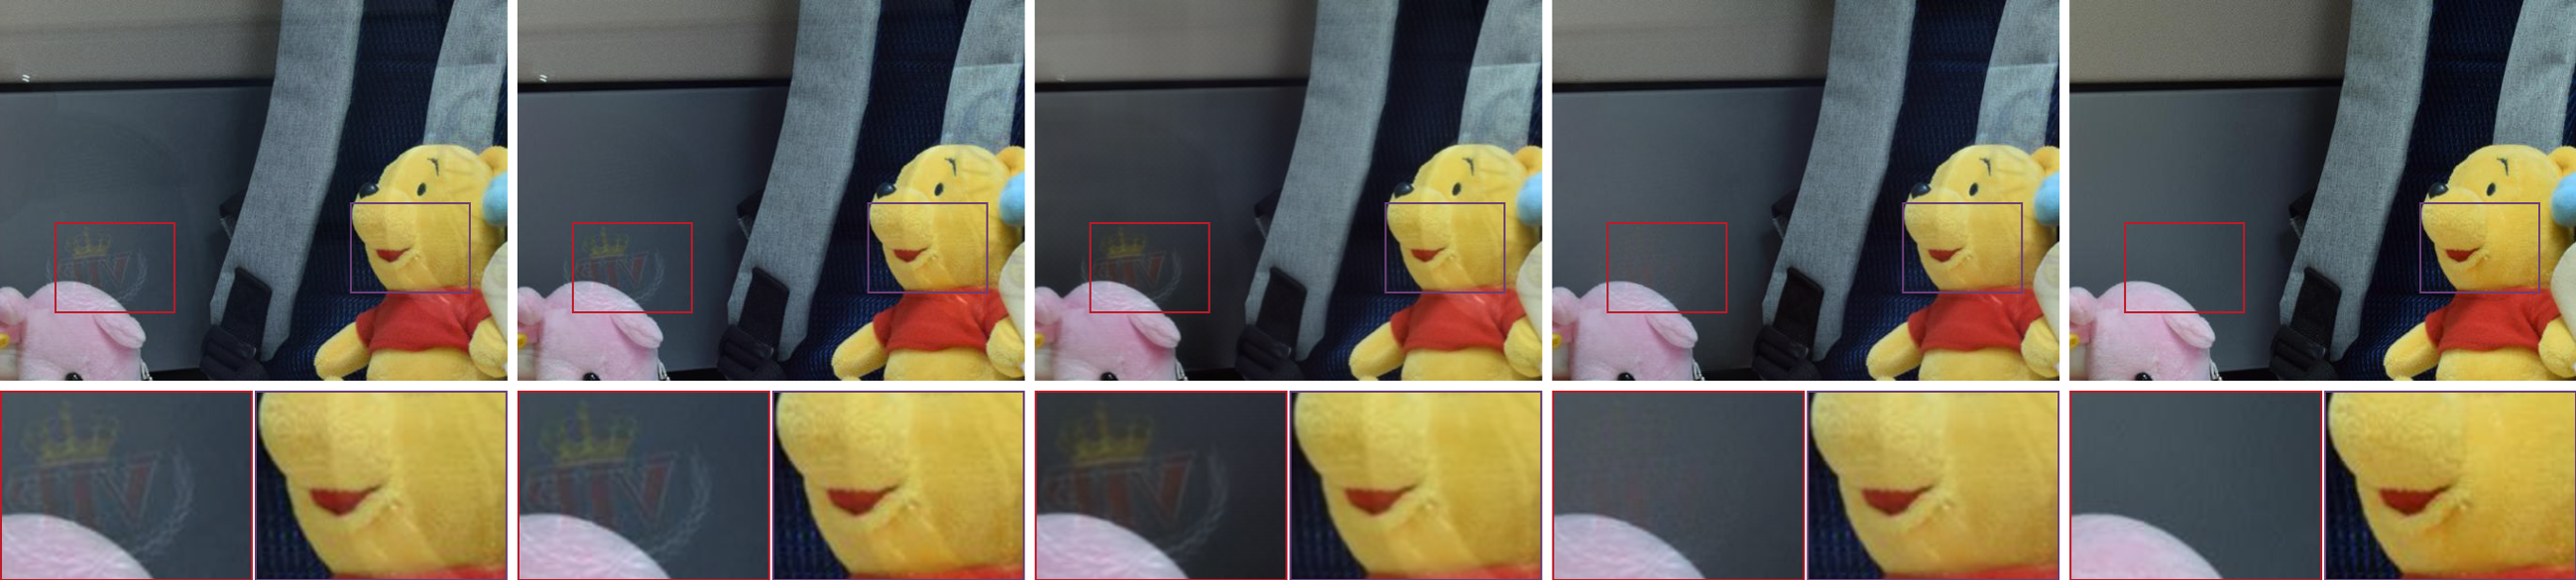}
    \includegraphics[width=\linewidth,height=3.5cm]{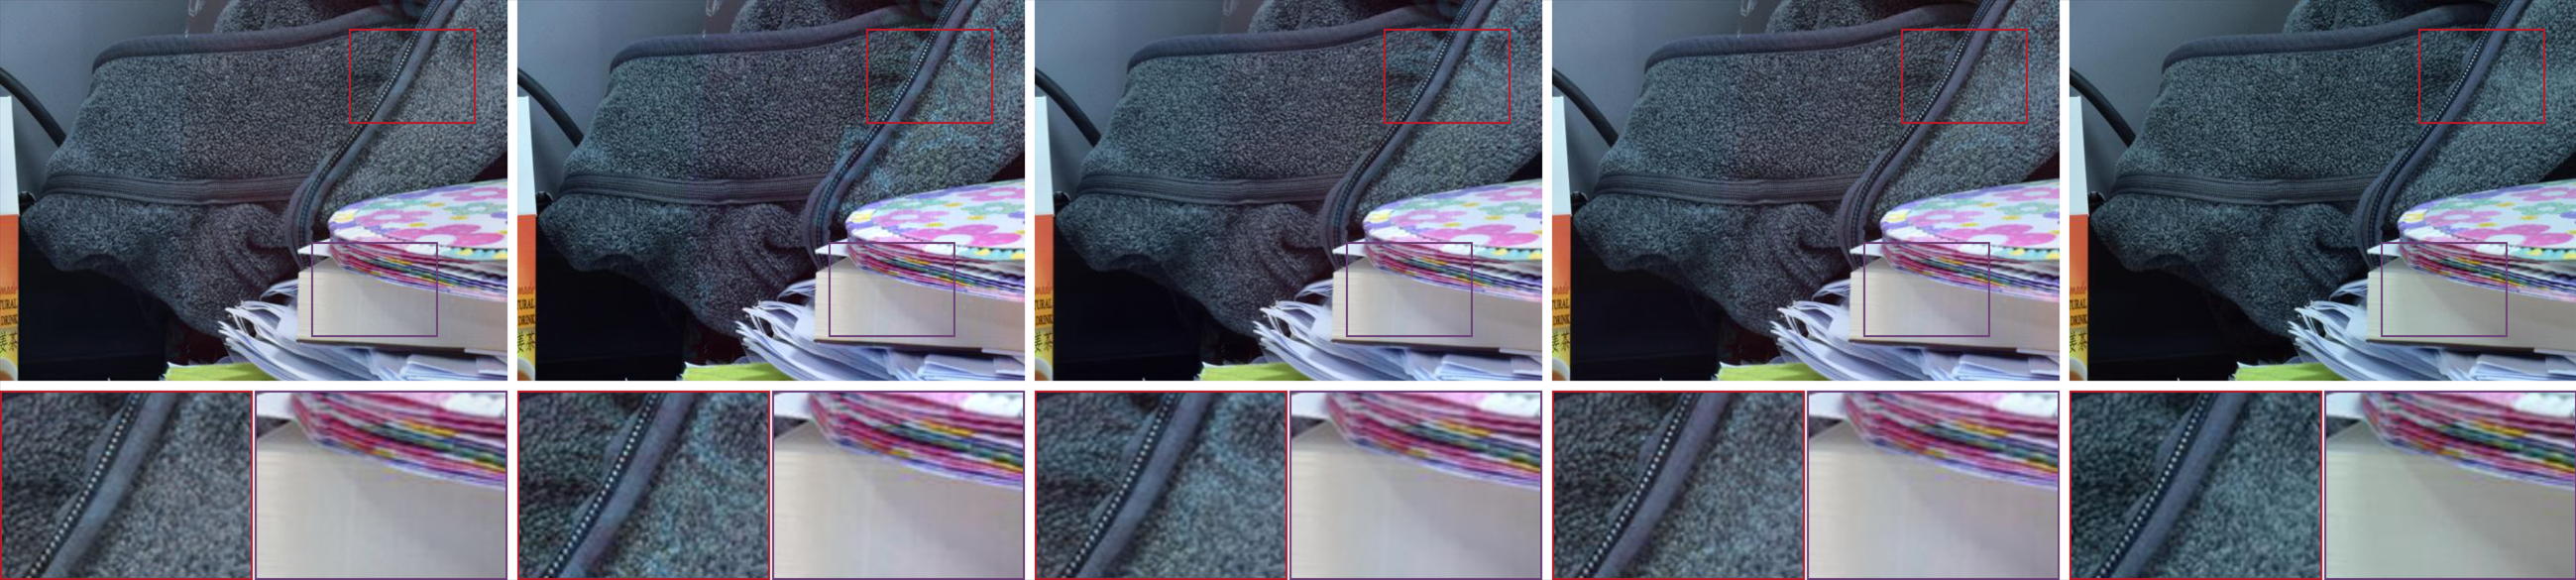}
    \begin{subfigure}{0.19\linewidth}
        \centering
        \subcaption{YTMT}
        \label{subfig:YTMT}
    \end{subfigure}
    \begin{subfigure}{0.19\linewidth}
        \centering
        \subcaption{DSRNet}
        \label{subfig:DSRNet}
    \end{subfigure}
    \begin{subfigure}{0.19\linewidth}
        \centering
        \subcaption{Zhu \textit{et al.}}
        \label{subfig:zhu}
    \end{subfigure}
    \begin{subfigure}{0.19\linewidth}
        \centering
        \subcaption{Ours}
        \label{subfig:input}
    \end{subfigure}
    \begin{subfigure}{0.19\linewidth}
        \centering
        \subcaption{GT}
        \label{subfig:input}
    \end{subfigure}
    
    \caption{Visual comparison of estimated transmission layers between state-of-the-arts and ours on Objects dataset.}
    \label{fig:Solid_appen}
\end{figure*}
\begin{figure*}[t]
    \centering
    \includegraphics[width=\linewidth,height=3.5cm]{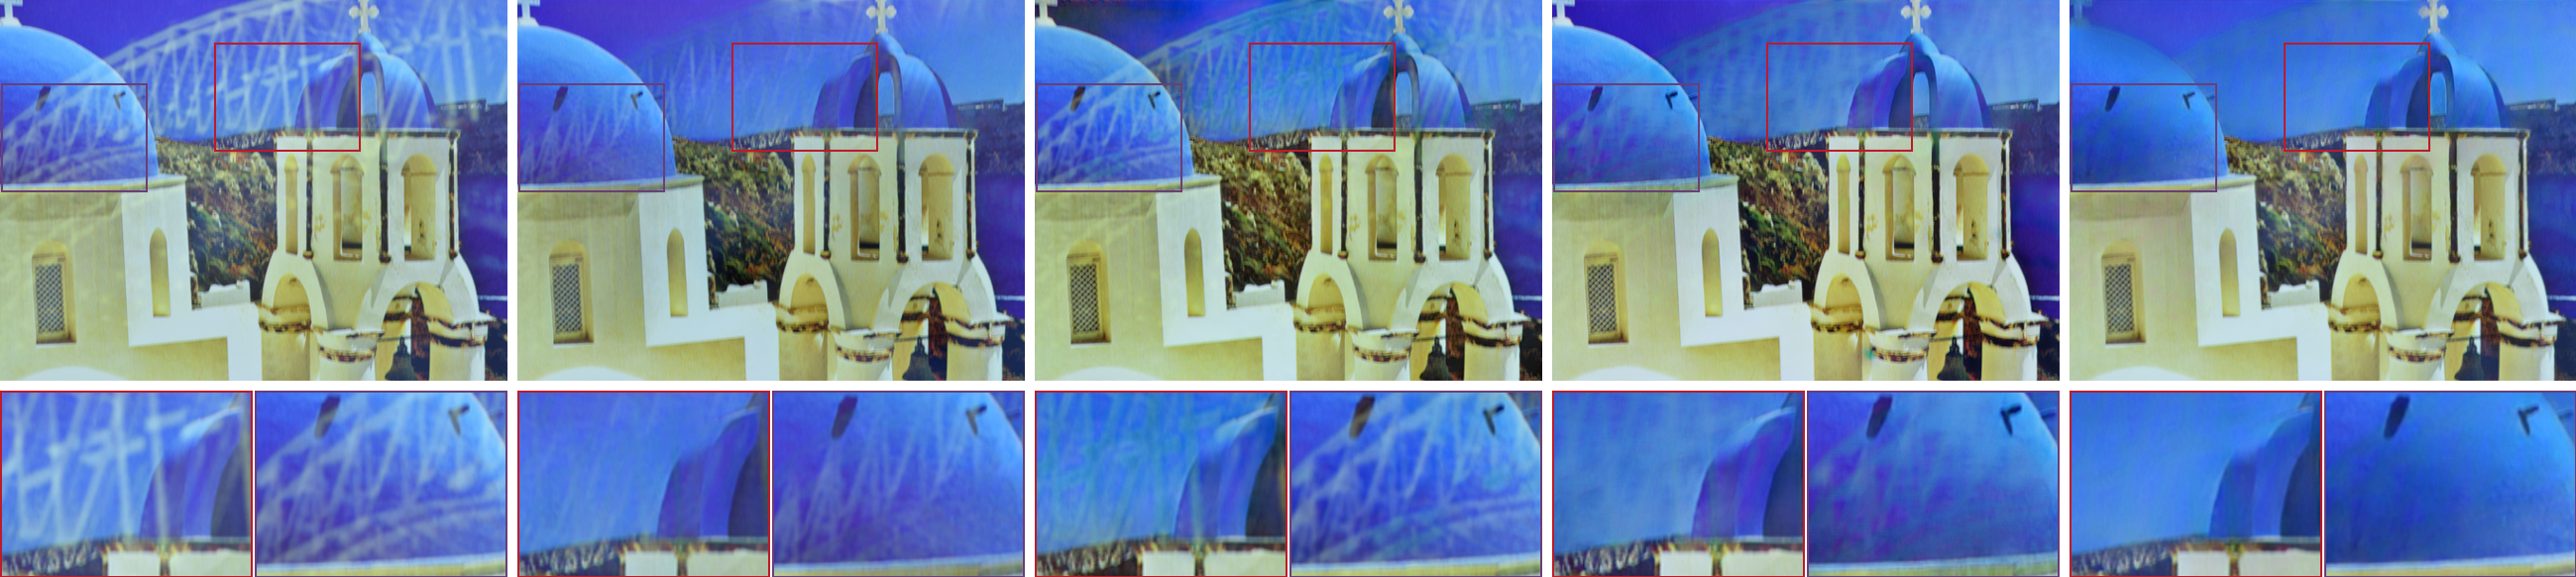} 
    \includegraphics[width=\linewidth,height=3.5cm]{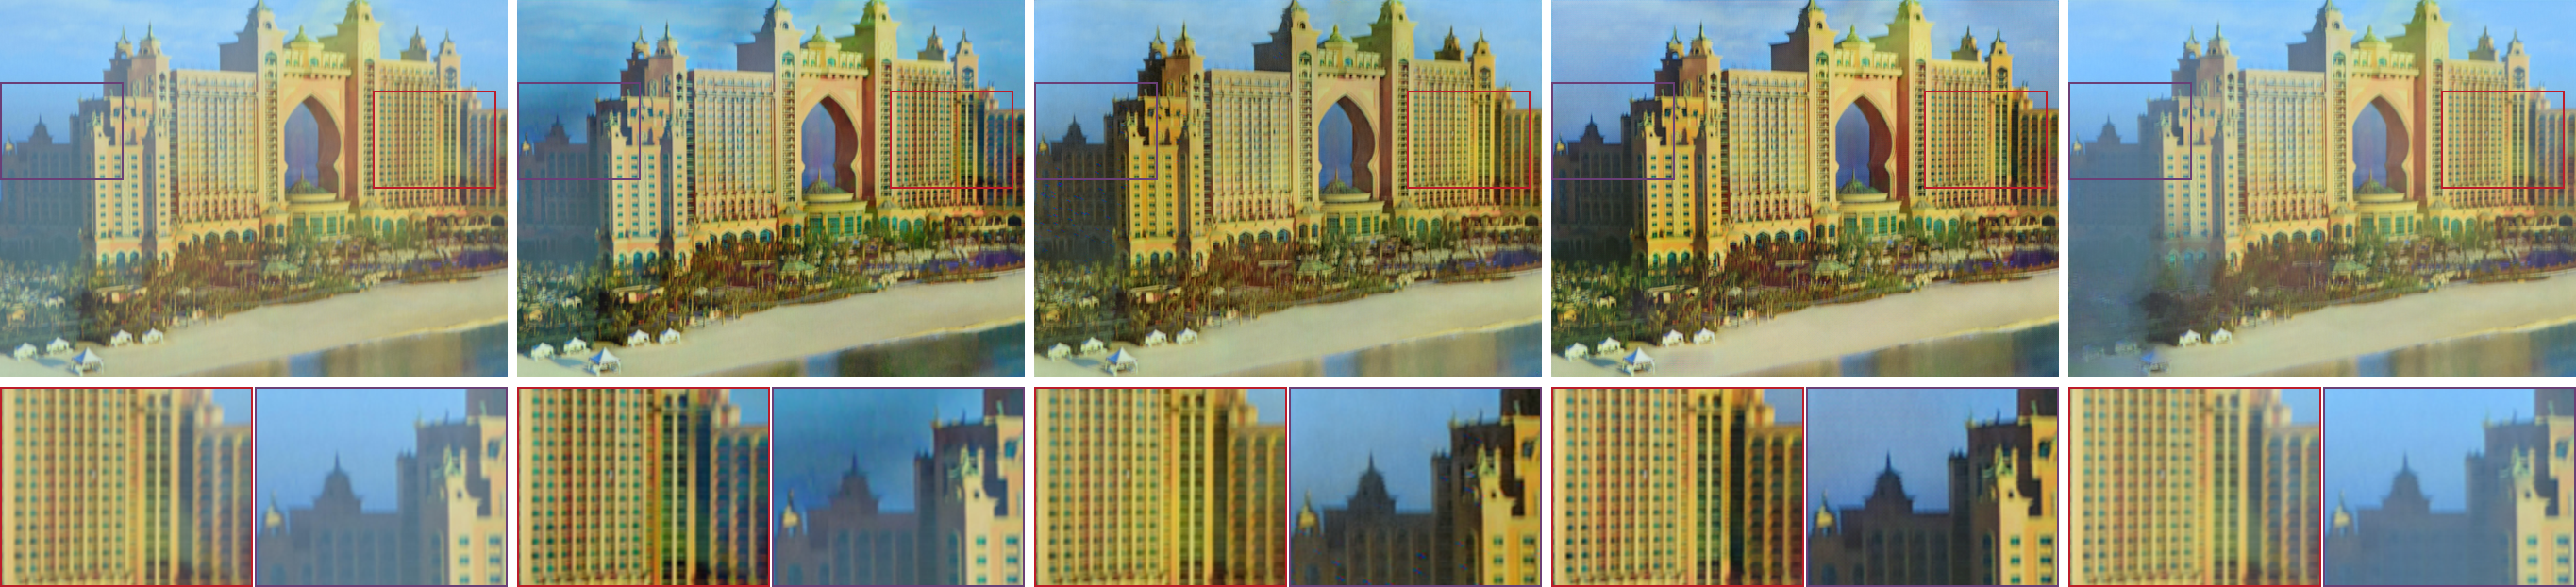}
    \includegraphics[width=\linewidth,height=3.5cm]{fig/sup_case6/stitch_images/Snipaste_2024-05-22_15-49-57.png}
    \begin{subfigure}{0.19\linewidth}
        \centering
        \subcaption{Input}
        \label{subfig:input}
    \end{subfigure}
    \begin{subfigure}{0.19\linewidth}
        \centering
        \subcaption{ERRNet}
        \label{subfig:ERRNet}
    \end{subfigure}
    \begin{subfigure}{0.19\linewidth}
        \centering
        \subcaption{IBCLN}
        \label{subfig:IBCLN}
    \end{subfigure}
    \begin{subfigure}{0.19\linewidth}
        \centering
        \subcaption{RAGNet}
        \label{subfig:RAGNet}
    \end{subfigure}
    \begin{subfigure}{0.19\linewidth}
        \centering
        \subcaption{Dong \textit{et al.}}
        \label{subfig:Dong}
    \end{subfigure}
    \includegraphics[width=\linewidth,height=3.5cm]{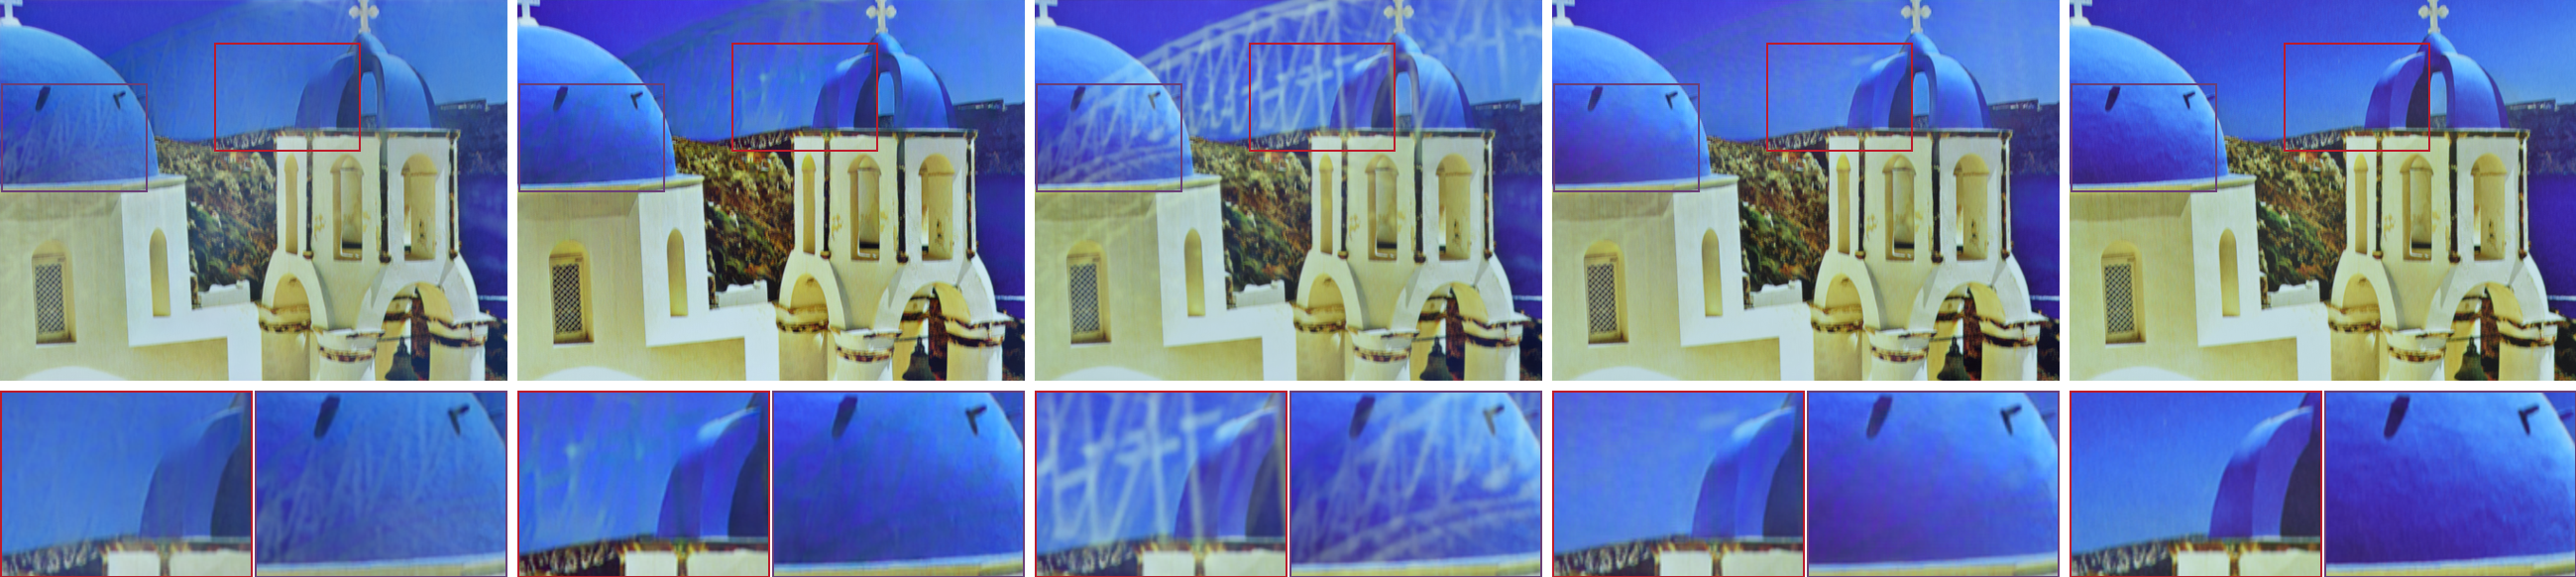}
    \includegraphics[width=\linewidth,height=3.5cm]{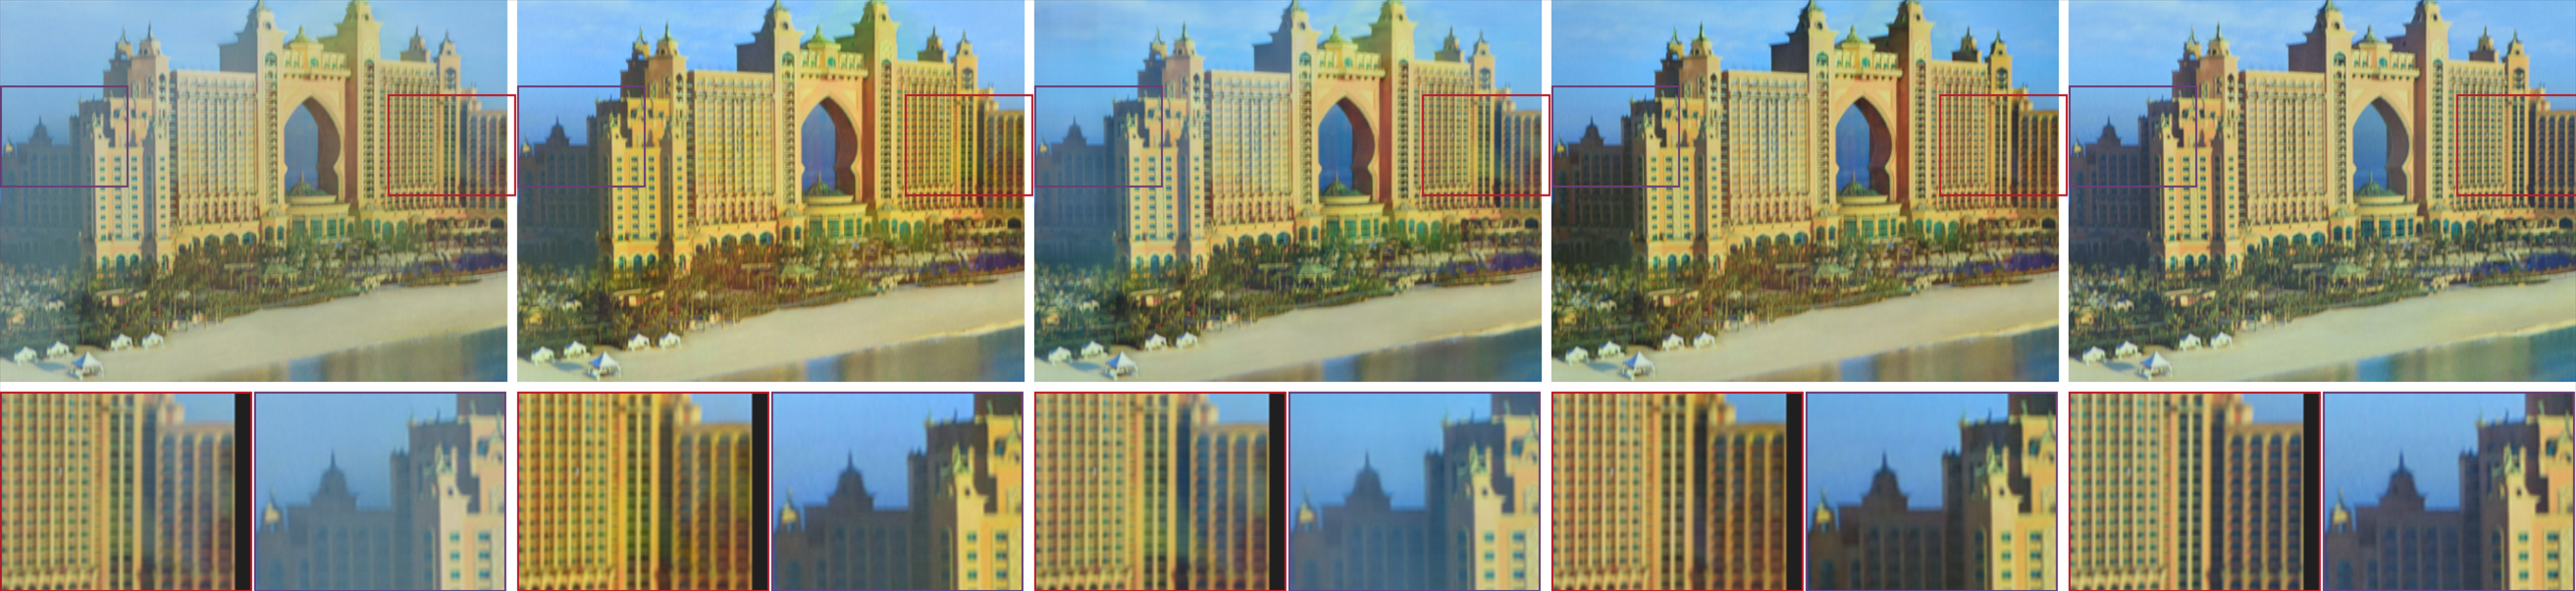}
    \includegraphics[width=\linewidth,height=3.5cm]{fig/sup_case6/stitch_images/5.png}
    \begin{subfigure}{0.19\linewidth}
        \centering
        \subcaption{YTMT}
        \label{subfig:YTMT}
    \end{subfigure}
    \begin{subfigure}{0.19\linewidth}
        \centering
        \subcaption{DSRNet}
        \label{subfig:DSRNet}
    \end{subfigure}
    \begin{subfigure}{0.19\linewidth}
        \centering
        \subcaption{Zhu \textit{et al.}}
        \label{subfig:zhu}
    \end{subfigure}
    \begin{subfigure}{0.19\linewidth}
        \centering
        \subcaption{Ours}
        \label{subfig:input}
    \end{subfigure}
    \begin{subfigure}{0.19\linewidth}
        \centering
        \subcaption{GT}
        \label{subfig:input}
    \end{subfigure}
    
    \caption{Visual comparison of estimated transmission layers between state-of-the-arts and ours on Postcard dataset.}
    \label{fig:Post_appen}
\end{figure*}
\begin{figure*}[t]
    \centering 
    \includegraphics[width=\linewidth,height=3.5cm]{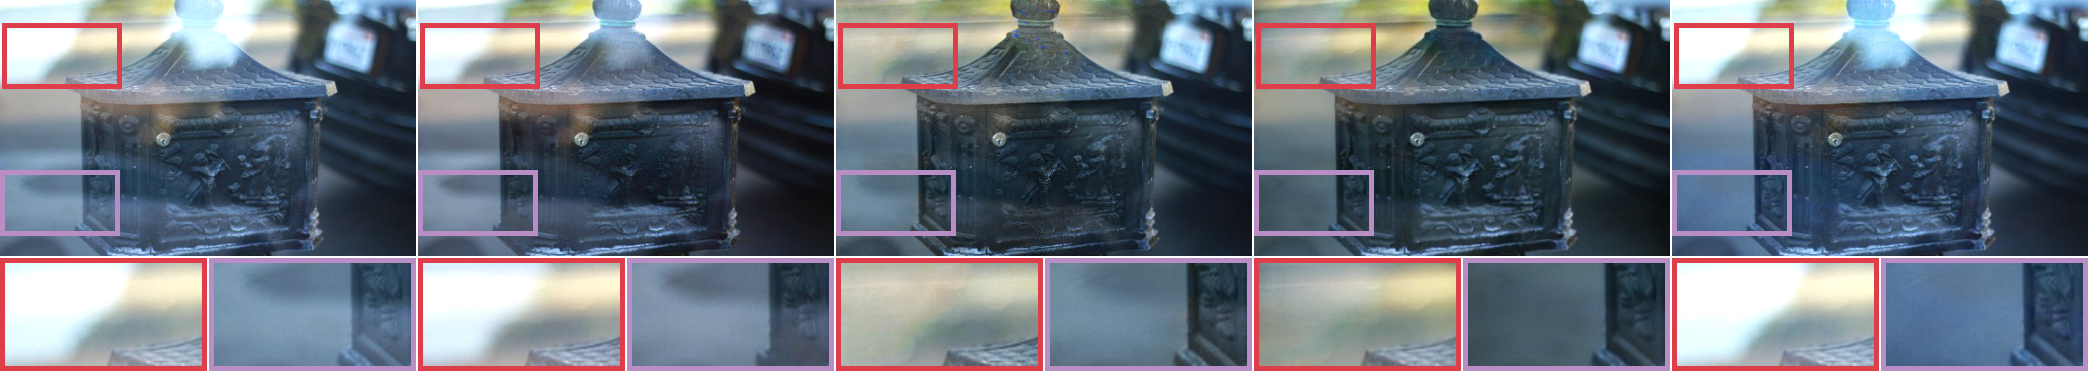}
    \includegraphics[width=\linewidth,height=3.5cm]{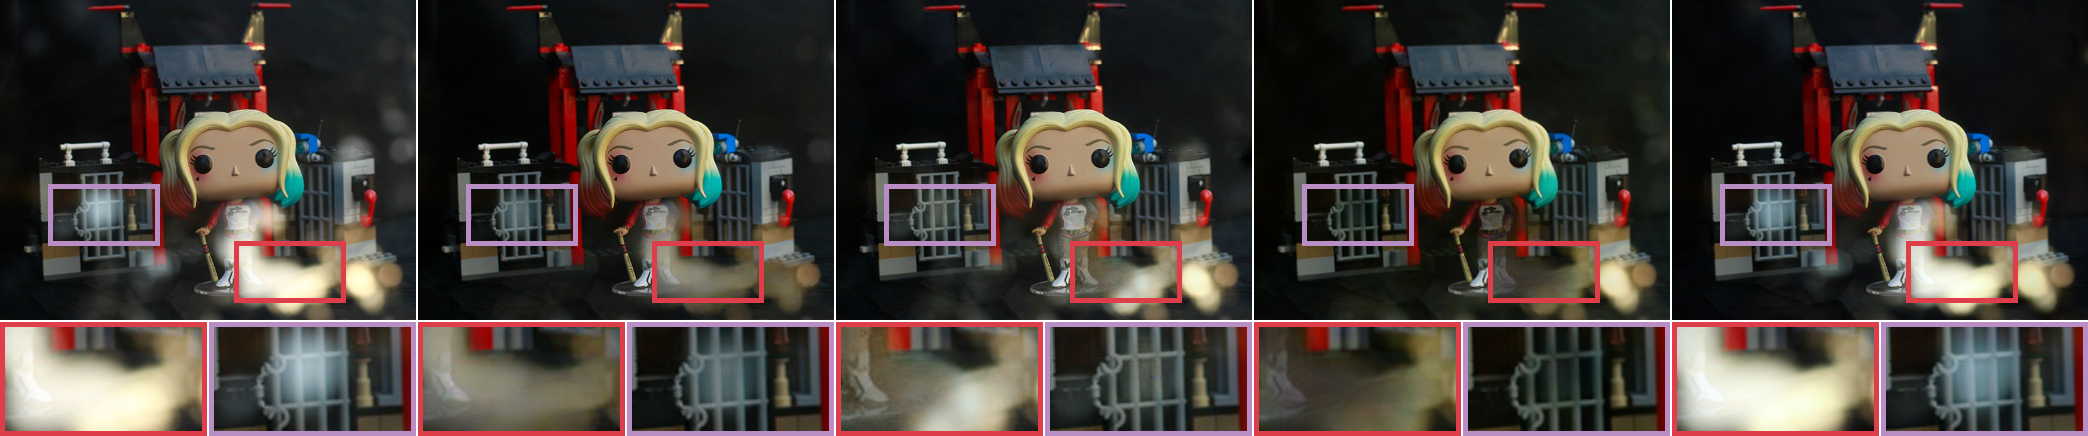}
    \begin{subfigure}{0.19\linewidth}
        \centering
        \subcaption{Input}
        \label{subfig:input}
    \end{subfigure}
    \begin{subfigure}{0.19\linewidth}
        \centering
        \subcaption{ERRNet}
        \label{subfig:ERRNet}
    \end{subfigure}
    \begin{subfigure}{0.19\linewidth}
        \centering
        \subcaption{IBCLN}
        \label{subfig:IBCLN}
    \end{subfigure}
    \begin{subfigure}{0.19\linewidth}
        \centering
        \subcaption{RAGNet}
        \label{subfig:RAGNet}
    \end{subfigure}
    \begin{subfigure}{0.19\linewidth}
        \centering
        \subcaption{Dong \textit{et al.}}
        \label{subfig:Dong}
    \end{subfigure}
    \includegraphics[width=\linewidth,height=3.5cm]{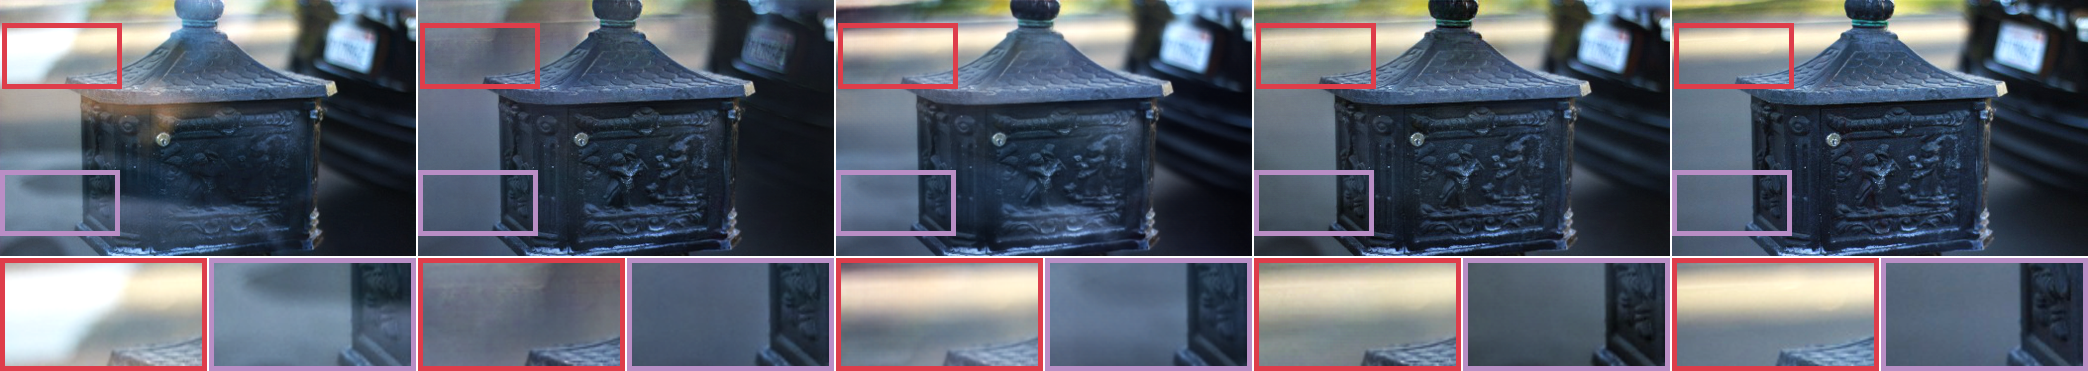}
    \includegraphics[width=\linewidth,height=3.5cm]{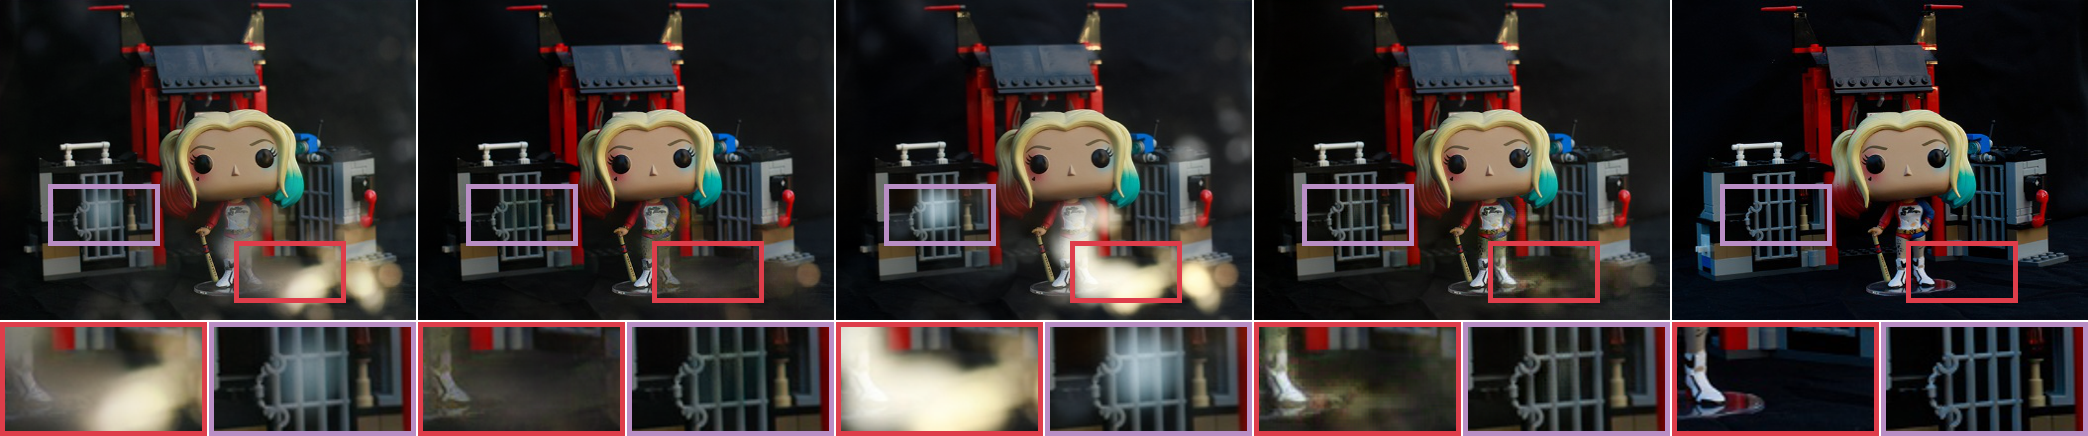}
    \begin{subfigure}{0.19\linewidth}
        \centering
        \subcaption{YTMT}
        \label{subfig:YTMT}
    \end{subfigure}
    \begin{subfigure}{0.19\linewidth}
        \centering
        \subcaption{DSRNet}
        \label{subfig:DSRNet}
    \end{subfigure}
    \begin{subfigure}{0.19\linewidth}
        \centering
        \subcaption{Zhu \textit{et al.}}
        \label{subfig:zhu}
    \end{subfigure}
    \begin{subfigure}{0.19\linewidth}
        \centering
        \subcaption{Ours}
        \label{subfig:input}
    \end{subfigure}
    \begin{subfigure}{0.19\linewidth}
        \centering
        \subcaption{GT}
        \label{subfig:input}
    \end{subfigure}
    
    \caption{Visual comparison of estimated transmission layers between state-of-the-arts and ours on real-world samples (Real 20).}
    \label{fig:real_appen}
\end{figure*}

\begin{figure*}[t!]
    \centering 
    \includegraphics[width=\linewidth]{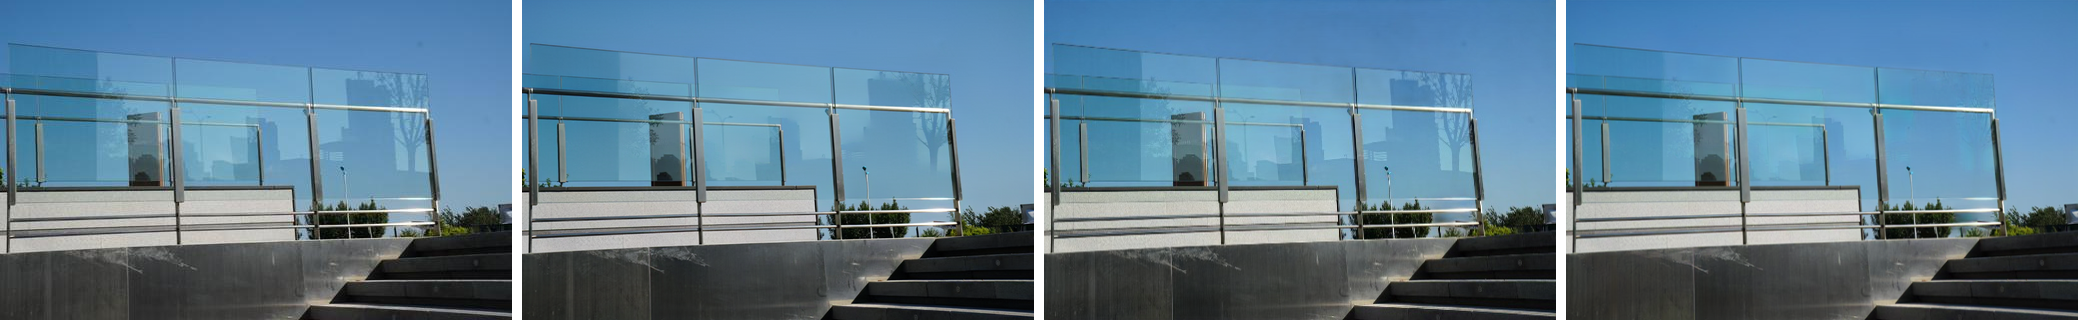}
    \includegraphics[width=\linewidth]{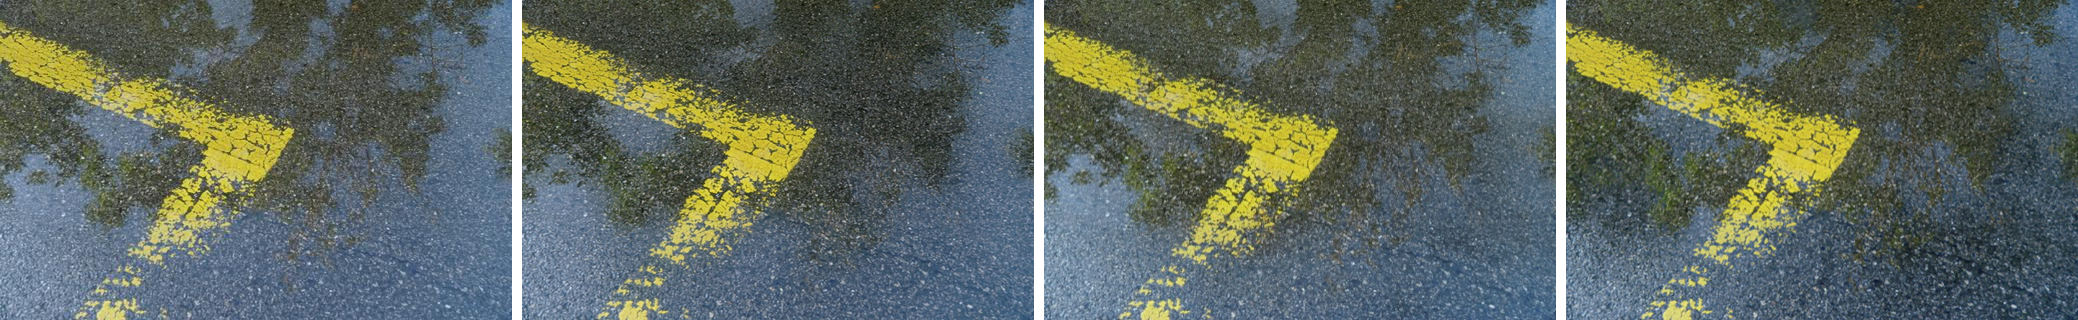}
    \begin{subfigure}{0.19\linewidth}
        \centering
        \subcaption{Input}
        \label{subfig:input}
    \end{subfigure}
    \begin{subfigure}{0.23\linewidth}
        \centering
        \subcaption{ERRNet}
        \label{subfig:ERRNet}
    \end{subfigure}
    \begin{subfigure}{0.23\linewidth}
        \centering
        \subcaption{IBCLN}
        \label{subfig:IBCLN}
    \end{subfigure}
    \begin{subfigure}{0.23\linewidth}
        \centering
        \subcaption{Dong \textit{et al.}}
        \label{subfig:Dong}
    \end{subfigure}
    \includegraphics[width=\linewidth]{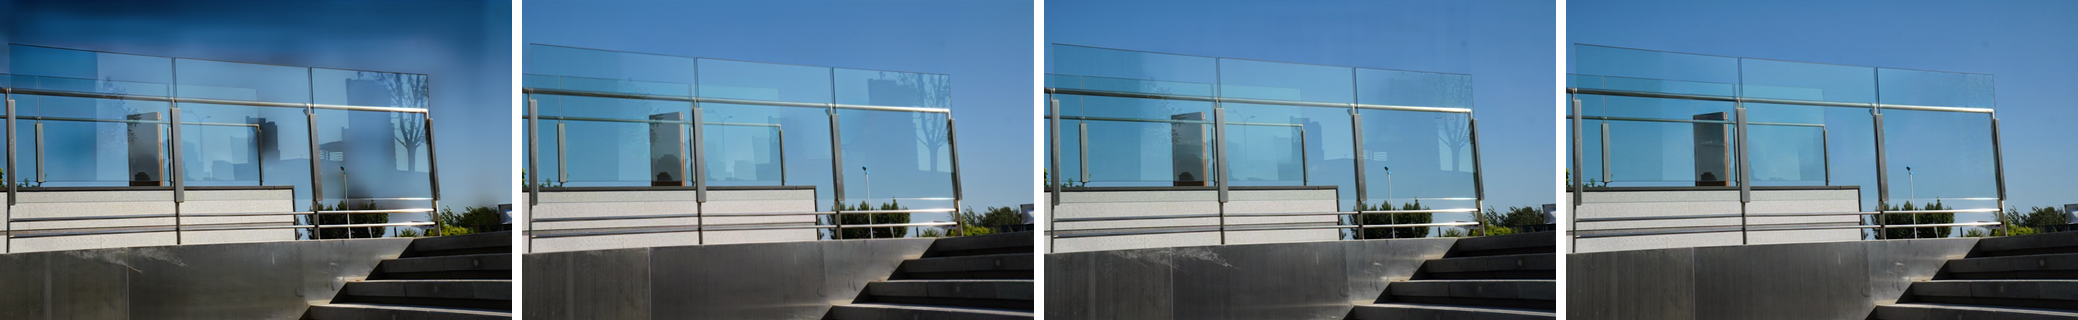}
    \includegraphics[width=\linewidth]{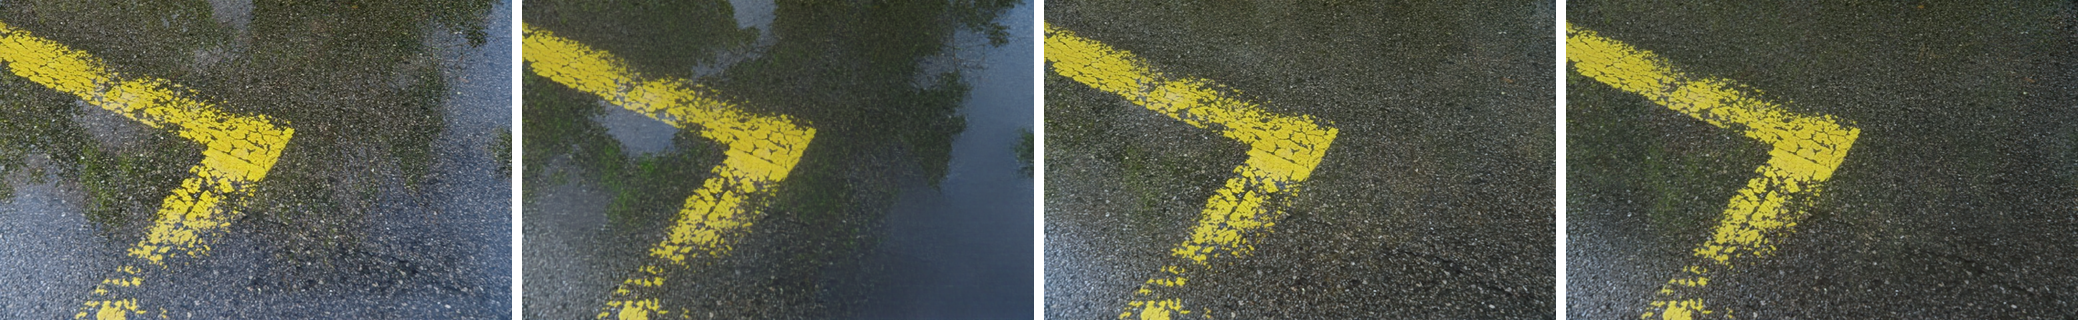}
    \begin{subfigure}{0.23\linewidth}
        \centering
        \subcaption{YTMT}
        \label{subfig:YTMT}
    \end{subfigure}
    \begin{subfigure}{0.23\linewidth}
        \centering
        \subcaption{DSRNet}
        \label{subfig:DSRNet}
    \end{subfigure}
    \begin{subfigure}{0.23\linewidth}
        \centering
        \subcaption{Zhu \textit{et al.}}
        \label{subfig:zhu}
    \end{subfigure}
    \begin{subfigure}{0.23\linewidth}
        \centering
        \subcaption{Ours}
        \label{subfig:input}
    \end{subfigure}
    \caption{Visual comparison of estimated transmission layers between state-of-the-arts and ours on real-world samples.}
    \label{fig:our_appen}
    
\end{figure*}

\begin{table}[t]
\centering
\resizebox{\columnwidth}{!}{
\begin{tabular}{lcccccc}
\toprule
    & ERRNet & IBCLN & YTMT & DSRNet & Zhu \textit{et al.} & Ours \\
\midrule[1pt]
PSNR & 22.18 & 23.57 & 23.85 & 25.22 & \underline{26.04} & \textbf{26.21} \\
SSIM & 0.756 & 0.783 & 0.810 & 0.832 & \textbf{0.846} & \underline{0.842} \\
\bottomrule
\end{tabular}
}
\caption{Quantitative results on the Nature dataset. The competitors are all trained with the additional data from the Nature dataset}
\label{tab:nature}
\end{table}
